# Supplementary material for: Manifold-constrained Gaussian process inference for time-varying parameters in dynamic systems
Source: arXiv:2105.13407 source file (2022-02-28)
Supplement: Supplementary file 1 [file SI.tex]

Novelty - difference in the problems of TVMAGI and MAGI. The seemingly small change in time-constant parameters  to time-varying parameters  in ODE in fact creates a huge difference in the scientific context, as most of the phenomena in real world are non-stationary or changing over time. From a technical stand point, with , the parameter estimation now becomes a functional estimation, which is much more challenging. Generally speaking, in dynamical systems, a seemingly small and benign change in the formulation could lead to drastically different system: PDE and ODE only differs in dimensionality, SDE and ODE only differs in stochastic component. In a similar argument, the problem of time-varying parameter should not be taken lightly or trivialized.

Novelty - difference in the methodology of TVMAGI and MAGI. The fact that we are able to find a simple and elegant solution doesn't mean the solution itself is trivial. TVMAGI extended on MAGI by introducing additional Gaussian Process in the time-varying parameters. The originality of TVMAGI to MAGI is just like Extended Kalman Filter to Kalman Filter, or Elastic Net to LASSO. On the note of borrowed content/context, it is our intention to keep the notations and theoretical framework consistent with MAGI for easier digest of the paper series. The underlying mathematical construct is very different: MAGI shows the proof for random variable , while TVMAGI works with stochastic process .

After all, novelty is a bit subjective. Even the four reviewers seem to hold different opinions. We appreciate this reviewer for pointing out that our "adjustment of MAGI to allow for time varying parameter inference ... is interesting and an important contribution" in the Significance section of the review. The rest of this response will focus on the concrete and actionable comments.

Re: Quality - The claims are only supported by 3 simulated examples, of which only the last includes comparisons with other methods.

Thanks for the good suggestion. We have added multiple baseline methods for comparison in all 3 simulated examples. These baseline methods fall into two classes (1) numerical integration method, represented by Runge-Kutta, and (2) Bayesian filtering methods including Extended Kalman Filter (EKF), Unscented Kalman Filter (UKF), Ensemble Kalman Filter (EnKF), and Ensemble Adjustment Kalman Filter (EAKF). The additional comparison results can be found in Section 2 of the newly added Supporting Information file https://www.overleaf.com/read/rrctcpgymtnv. We plan to add these results into the main paper during revision.

The key take-away with the baseline comparisons are:

TVMAGI is much faster and more accurate than the numerical integration method based on Runge-Kutta.
Bayesian filtering method is the fastest, but gives unreliable results with terrible accuracy. A discussion on why Bayesian filtering would fail is included in the Section 3 of the link above, and also included in the specific response letter to reviewer "dBwN".
Re: Section 4 discusses exactly what steps are take to obtain the MAP estimate, but does not discuss why.

We thank the reviewer for pointing out this oversight in the paper writing. We plan to add the following explanation to the reason of carrying out multi-stage optimization during the revision at the beginning of Section 4.

"The multi-stage optimization is introduced for three reasons. (1) The GP hyperparameters 
 for the system components are set at the first stage and hold as constant in the rest of the optimization so that kernel matrix inverse only needs to be computed once, following the recommendation of Ref.[8]. (2) The GP hyperparameters 
 for the time-varying parameters could not be set without any information about , so a feedback procedure is designed, where a point-wise 
 is obtained in one stage without GP, and then GP hyperparameters 
 is estimated in the following stage based on 
. (3) The multi-stage optimization ensures that each step of the optimization starts with sensible initial value obtained from previous modularized optimization, thus drastically decreasing the chance of Adam optimizer stuck in local mode. Experiments have shown that the carefully designed multi-stage optimization achieves better results than joint optimization with much faster speed."

Re: The experiments show good performance of TVMAGI, but the first two experiments do not have any baseline comparison

We have added multiple baseline methods for comparison in all 3 simulated examples. Please refer to the earlier reply for details.

Re: No timing was included for the HIV experiment comparing with state-of-art method

We have added a computation time table for comparisons with additional baseline methods and the state-of-art benchmark method. Please see Table 5 in the newly added Supporting Information file https://www.overleaf.com/read/rrctcpgymtnv. Our TVMAGI is shown to be faster than baseline methods of Runge-Kutta.

TVMAGI has slightly better accuracy than the state-of-art benchmark method of Efficient Local Estimation in Ref.[13], and TVMAGI is also much more generally applicable than the benchmark method. However, TVMAGI comes with the expense of longer computing time compared with benchmark [13], which is tailor made for the HIV example.

Re: The experiments do not explore the sensitivity

Matern kernel with degree of freedom  is chosen for system components because it is the simplest kernel that ensures continuous differentiable curve, which is minimally required for the ODE. We agree that the GP kernel for the time-varying parameter could be even more relaxed. We also agree additional sensitivity analysis on the number of discretization points would be helpful to understand the robustness of TVMAGI.

We have conducted two additional sensitivity analysis. (1) Relax the GP kernel of time-varying parameter  to be Matern kernel with degree of freedom , i.e.,  is required to be continuous, but not necessarily differentiable, allowing for more abrupt changes. (2) Experiments with different number of discretization points. We recommend gradually increase the number of discretization points until result converges. Note the convergence is ensured by our theoretical derivation. However, increasing number of discretization points will linearly increase the computational time.

Full results on sensitivity analysis can be found in Section 4 in the newly added Supporting Information file https://www.overleaf.com/read/rrctcpgymtnv. We found the TVMAGI to be insensitive to the GP kernel or the number of discretization through the SEIRD experiment. In fact, the result got slightly better when Matern kernel with degree of freedom  is used on  for SEIRD.

On the issue of ADAM getting stuck in local maximums, we used a carefully designed multi-stage optimization procedure to achieve the final MAP, thus alleviating the concern. We have compared our MAP with that obtained with randomized starting value for Adam optimization. We found our multi-stage optimization procedure to always be much closer to the ground truth, while randomized starting value for Adam optimization will often get stuck in local maximums and thus yield insensible results. Please see earlier reply on the reason of proposed multi-stage optimization.

Re: Worse sensitivity when 
 & Picking kernel for  to prevent overfitting

The sensitivity issues getting worse when 
 mostly with optimization, which is the reason why we proposed a much more elaborated multi-stage optimization procedure in TVMAGI. The over-fitting issue on  can be prevented by (1) a Matern  kernel that ensures continuously differentiable , which prevents  from fitting white noise, and (2) setting a prior lower bound on the length-scale (a.k.a. bandwidth) hyperparameters 
 of GP for . The Matern  kernel together with prior on the length-scale hyperparameter ensures the smoothness and the degree of variability in , which in turn prevents overfitting.

Re: Clarity & Significance

We thank the reviewer for the appreciation of our clarity and our contribution. The comments are insightful and constructive. We believe our paper is in better shape after incorporating reviewer's suggestion.
